# Supplementary material for: Do LLMs Understand Visual Anomalies? Uncovering LLM's Capabilities in Zero-shot Anomaly Detection
Source: arXiv:2404.09654 source file (2025-04-07)
Supplement: Supplementary file 1 [file 7_suppl.tex]

\clearpage
\setcounter{page}{1}
\maketitlesupplementary
% \onecolumn
% \centerline{\Large{\textbf{\thetitle}}\\ \vspace{0.5em}}
% \centerline{\Large{Supplementary Material}}

\section{Implementation details}
\label{sec:implementation_details}

\noindent
\textbf{Data pre-processing.}
% follow~\cite{jeong2023winclip,deng2023anovl}, data augment 
We employ the data pre-processing pipeline outlined in the OpenCLIP implementation~\cite{ilharco_gabriel_2021_5143773} for both the MVTec~\cite{bergmann2019mvtec} and VisA~\cite{zou2022spot} benchmarks.
This process entails channel-wise standardization using the pre-computed mean [0.48145466, 0.4578275, 0.40821073] and standard deviation [0.26862954, 0.26130258, 0.27577711] after normalizing each RGB image to [0, 1]. 
Subsequently, we apply bicubic resizing based on the Pillow implementation (PIL).
% By default, we make the input resolution 240 for the shorter edge from the re-sizing, to be compatible with ViT-B/16+ in our experiments. 
% This re-sizing policy also applies to other baseline models for fairer comparisons, although we keep the remaining parts of their original data pre-processing pipelines. 
% In addition, the similar policy can also be used in other backbones with the input of different resolutions.
We note that CLIP requires a square-shaped resolution for input image queries.
To adapt CLIP to non-square images in the VisA benchmark, we employ an ``image tiling" scheme, as suggested by \cite{jeong2023winclip}.
The resizing policy is also adopted for other baseline models to ensure fair comparisons, while the remaining parts of their original data pre-processing pipelines are retained.

\noindent
\textbf{Anomaly prompt generation via unified templates.}
% we formulate a unified template decomposing the prompting engineering into several components to generate the contrastive-state prompts as: ``A \{\textit{domain}\} image of a \{\textit{state}\} \{\textit{class}\} [with \{\textit{specific details}\}].".
Recall that we formulate a unified template to generate the contrastive-state prompts as: ``A \{\textit{domain}\} image of a \{\textit{state}\} \{\textit{class}\} [with \{\textit{specific details}\}].", where ``class" in the template is replaced by the class name in MVTec and VisA benchmarks.
Along this line, we perform prompt enhancement by replacing some fixed words in the template such as ``image" with ``photo". 
Additionally, given the potential ambiguity of certain class names, such as ``bottle" in MVTec and ``pcb1" and ``pcb2" in VisA, we opted to substitute these class names in the original dataset with more specific object names or concise descriptions.
% Additionally, we use the object name words available for both MVTec and VisA per dataset to replace ``class" in the template.
% Figure~\ref{} provides a detailed list of prompts we adopt in this work.
We present a sample list of templates utilized in this study, denoted as:
templates = [
    ``an image of a \{$\Omega$\}",
    ``a close-up image of a \{$\Omega$\}",
    ``an industrial image of a \{$\Omega$\}",
    ``a manufacturing image of a \{$\Omega$\}",
    ``a production image of a \{$\Omega$\}",
    ``a textural image of a \{$\Omega$\}",
    ``a surface image of a \{$\Omega$\}",
    ``a cross-section image of a \{$\Omega$\}"
]. Here, ``\{$\Omega$\}" represents a description of the contrastive state of a specific class. 

Specifically, we formulate ``\{$\Omega$\}" as: 
normal state = [``$\varsigma$",
                ``normal $\varsigma$",
                ``undamaged $\varsigma$",
                ``flawless $\varsigma$",
                ``perfect $\varsigma$",
                ``unblemished $\varsigma$",
                ``$\varsigma$ without flaw",
                ``$\varsigma$ without defect",
                ``$\varsigma$ without damage",
                ]
and
abnormal state = [``abnormal $\varsigma$",
                  ``damaged $\varsigma$",
                 ``flawed $\varsigma$",
                 ``imperfect $\varsigma$",
                 ``impaired $\varsigma$', 
                 ``blemished $\varsigma$",
                 ``$\varsigma$ with flaw",
                 ``$\varsigma$ with defect",
                 ``$\varsigma$ with damage"],
where $\varsigma$ represents the class name in the benchmarks.

\noindent
\textbf{Anomaly prompt generation via an LLM.}
The LLM-based prompt generation is constrained to a maximum of 50 tokens.
The temperature is set to 0.9 to generate diverse and creative prompts while avoiding duplicate prompts.
The input query fed to the LLM typically follows the format: ``Describe what the image will look like if there is an anomaly in the image of $\varsigma$".
We aim for syntactic alignment between LLM-generated prompts and template-generated prompts by incorporating the instruction "Please state the description beginning with: An abnormal image of $\varsigma$." into the input query for the LLM. 
For the class name, we use the same operation as for the template-generated prompts to replace the ambiguous class name with a more comprehensible one for the LLM.
% Further experimental setup details and more discussion about prompts, including the prompts list considered in this paper, are available in Appendix.
%All the prompts are presented in appendix.

% \begin{figure*}[t]
%     \centering \vspace{-4mm}
%     \includegraphics[width=0.9\linewidth]{figs/}  
%     \caption{List of prompts generated using the unified template.
%     }
%     \label{fig:prompt_list}
%     \vspace{-3mm}
% \end{figure*}

\noindent
\textbf{Baseline.}
In our evaluation, \name is compared to various state-of-the-art methods in zero-shot, few-shot, and full-shot regimes, spanning image-level and pixel-level anomaly detection, including CLIP-AC~\cite{radford2021learning}, Trans-MM~\cite{chefer2021generic}, WinCLIP~\cite{jeong2023winclip}, AnoVL~\cite{deng2023anovl}, PatchCore~\cite{roth2022towards}, PaDiM~\cite{defard2021padim}, JNLD~\cite{zhao2022just}, UniAD~\cite{you2022unified}, AnomalyGPT~\cite{gu2023anomalygpt}, and SAA+~\cite{cao2023segment}, underlining its competitiveness across diverse benchmark scenarios.
% In zero-shot regime, we compare \name with CLIP-AC~\cite{radford2021learning} for image-level anomaly detection, Trans-MM~\cite{chefer2021generic} for pixel-level anomaly detection, and WinCLIP~\cite{jeong2023winclip} and AnoVL~\cite{deng2023anovl} for both image-level and pixel-level anomaly detection. 
% In the few-shot regime, we benchmark \name against PatchCore~\cite{roth2022towards} and WinCLIP~\cite{jeong2023winclip}.
% Additionally, we benchmark \name against prominent unsupervised and finetune-required VAD methods in a unified setting for fairness.
% Most baselines undergo training or finetuning on normal samples encompassing all classes within the dataset. 
% Moreover, we include two full-shot training-free methods, PatchCore~\cite{roth2022towards} and SAA+~\cite{cao2023segment}.
A brief introduction and reproduction details are given as follows.

CLIP-AC~\cite{radford2021learning}, WinCLIP~\cite{jeong2023winclip}, AnoVL~\cite{deng2023anovl}, and AnomalyGPT~\cite{gu2023anomalygpt} are variants built upon the CLIP designed for the unified training paradigm.
CLIP-AC~\cite{radford2021learning} refers to the original CLIP zero-shot classification extended with prompts of the form ``normal {class}" and ``anomalous {class}" using a prompt ensemble.
WinCLIP~\cite{jeong2023winclip} is a window-based CLIP variant featuring a compositional ensemble of state words and prompt templates and using sliding windows for dense visual feature extraction.
% AnoVL~\cite{deng2023anovl} introduces a training-free adaptation via value-to-value attention to obtain local patch features. It also proposes a test-time adaptation which is a learnable residual-like adapter to improve the performance of anomaly localization.
AnoVL~\cite{deng2023anovl} introduces a training-free adaptation through value-to-value attention for local patch features and a test-time adaptation using a learnable residual-like adapter to enhance anomaly localization performance. 
AnomalyGPT~\cite{gu2023anomalygpt} generates training data by simulating anomalous images, providing fine-grained semantics through an image decoder, and fine-tuning the LVLM with prompt embeddings using a prompt learner.
CLIP-AC and WinCLIP results are reported from~\cite{jeong2023winclip}, while the results for AnoVL\footnote{\url{https://github.com/hq-deng/AnoVL}} and AnomalyGPT\footnote{\url{https://github.com/CASIA-IVA-Lab/AnomalyGPT}} are executed using publicly available implementations.
% CLIP-AC and WinCLIP results are reported from the original paper~\cite{jeong2023winclip} as the method is not open source

There are four additional unified visual anomaly detection approaches.
Trans-MM~\cite{chefer2021generic} is a model interpretation method for Transformers, offering pixel-level masks for anomaly localization.
% Trans-MM~\cite{chefer2021generic} is a model interpretation method for Transformers, offering pixel-level masks for anomaly localization.
PatchCore~\cite{roth2022towards} introduces a maximally representative memory bank of neighborhood-aware patch features obtained from an encoder pre-trained on ImageNet.
% SAA+~\cite{cao2023segment} assemble these models to harness diverse multi-modal prior knowledge for anomaly localization, leveraging the strong zero-shot generalization ability of foundation models, such as the language-driven visual grounding model GroundingDINO and the prompt-driven segmentation model SAM. It also introduces hybrid prompts that incorporate domain expert knowledge and target image context as regularization.
SAA+~\cite{cao2023segment} introduces hybrid prompts regularization to incorporate domain expert knowledge and integrates models like GroundingDINO and SAM, leveraging their strong zero-shot generalization, to harness diverse multi-modal prior knowledge for anomaly localization.
UniAD~\cite{you2022unified} proposes a feature reconstruction framework consisting of a neighbor-masked encoder and a layer-wise query decoder to facilitate the model escape from the identity shortcut.
In the unified case, Trans-MM\footnote{\url{https://github.com/hila-chefer/Transformer-Explainability}}, PatchCore\footnote{\url{https://github.com/amazon-science/patchcore-inspection}}, SAA+\footnote{\url{https://github.com/caoyunkang/Segment-Any-Anomaly}}, and UniAD\footnote{\url{https://github.com/zhiyuanyou/UniAD}} are executed using publicly available implementations.

Additionally, PaDiM~\cite{defard2021padim} and JNLD~\cite{zhao2022just} are both ``one-class-one-model” methods, employing a separate training scheme. The former utilizes a pre-trained convolutional neural network (CNN) for patch embedding and employs multivariate Gaussian distributions to model the probabilistic representation of the normal class.
The latter comprises an anomaly reconstruction sub-network and a segmentation sub-network, both structured as encoder-decoder architectures, aiming to localize anomalies through the generated multi-scale anomalies.
For fairness, we obtain the results of PaDiM and JNLD from~\cite{gu2023anomalygpt}
% by training their models using the publicly available implementations
, following the unified paradigm of one model across all classes in the benchmark.

\noindent
\textbf{Experimental Environment.}
% \textbf{Other implementation details.}
%\subsubsection{\blue{Experimental Environment.}}
%X2
All the experiments are conducted in a server with Xeon(R) Silver 4214R CPU @ 2.40GHz (12 cores), 128G memory, and GeForce RTX 3090.
All the models are implemented in PyTorch 2.0.0 with CUDA 11.8.

%We apply WinCLIP with stride 1 on ViT patch embeddings, which is equivalent to stride 16 in pixel-level in case of ViT-B/16+.

\noindent
Our code is available at \url{https://anonymous.4open.science/r/LEAD-7613/}

\begin{figure}[t]
    \centering
    % \vspace{-2mm}
    \includegraphics[width=1\linewidth]{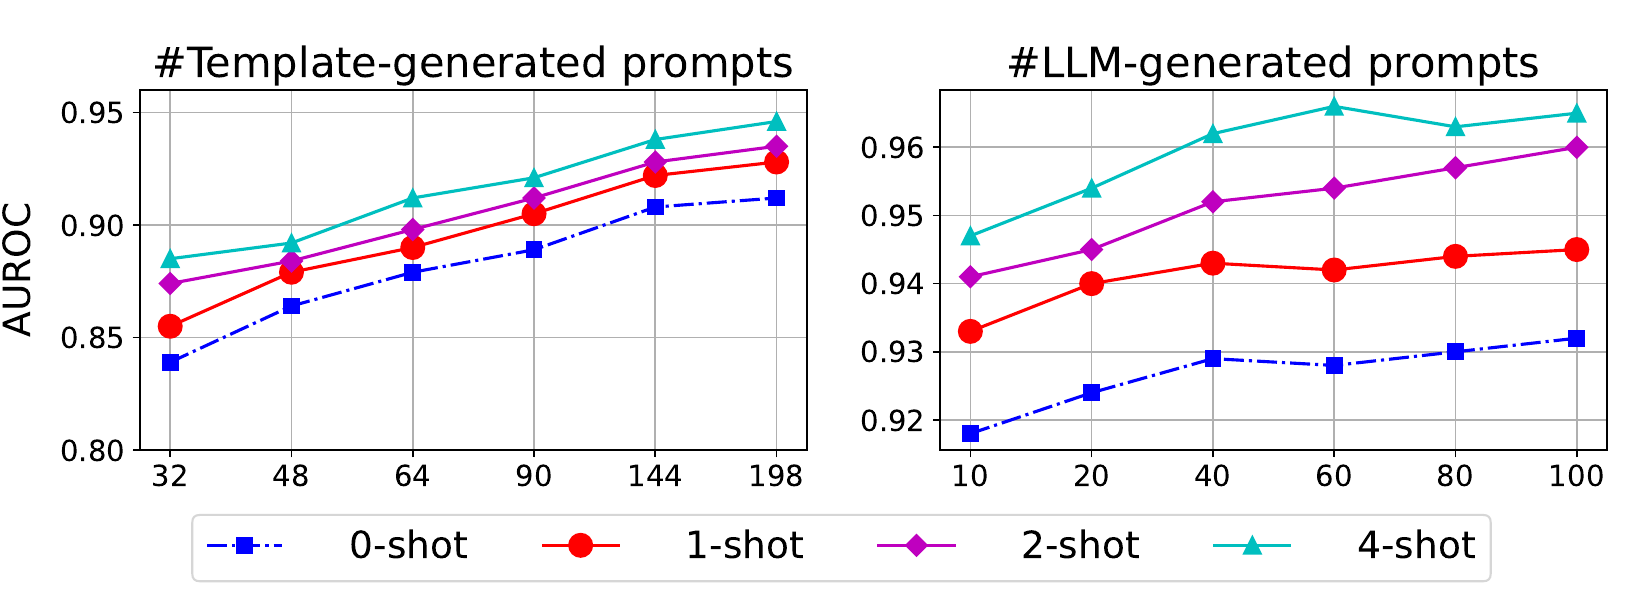}
    \caption{Effect of varying the number of anomaly prompts generated by templates and LLM on MVTec.
    }
    \label{fig:sup_prompt}
     \vspace{-2mm}
\end{figure}

\section{Additional results on ablation study}
\label{sec:add_ablation}
\noindent
\textbf{Effect of varying anomaly prompt quantities.}
In Figure~\ref{fig:sup_prompt}, we assess the impact of varying the number of prompts generated by both templates and LLM.
First, we evaluate the performance solely based on the anomaly prompts generated by templates. 
Our findings reveal a notable improvement in performance in both zero-shot and few-shot scenarios with an increasing number of template-generated anomaly prompts, as illustrated in the right subfigure of Figure~\ref{fig:sup_prompt}.

Building upon this, we introduce the anomaly prompts generated by an LLM and evaluate their impact with varying quantities.
We observed that the LLM-generated anomaly prompts can further improve the performance, even when it has already reached advanced stages.
Moreover, with an increasing number of LLM-generated anomaly prompts, performance gradually improves. However, the rate of improvement progressively slows down and may exhibit slight oscillations.
Therefore, we adopt a combination of 198 template-generated anomaly prompts and 100 LLM-generated anomaly prompts in our study.

\noindent
\textbf{Scalability.}
We evaluate the effect of various LAION-400M-based CLIP pre-trained models available at OpenCLIP\footnote{\url{https://github.com/mlfoundations/open_clip}}, as detailed in Table~\ref{tab:scalability}. 
Given that different backbones are associated with distinct input image sizes, we implement a unified data pre-processing procedure, employing bicubic resizing based on PIL, as described in Section~\ref{sec:implementation_details}.
We note that larger models or resolutions contribute to improved performance, thus we choose ViT-B/16+ with increased resolution as our default backbone.

\begin{table}[t!]
    \small
    \centering
    
    \caption{ Scalability analysis of \name on MVTec. }
    % \vspace{-2mm}
    \label{tab:scalability}
    \resizebox{0.9\columnwidth}{!}{
        \begin{tabular}{ c c c c c c c }
    \toprule[1.5pt]
   \multicolumn{3}{c}{Backbone} &  \multicolumn{4}{c}{$\#$shot (AUROC)}\\
   \cmidrule(lr){1-3} \cmidrule(lr){4-7}
   Model & Image Size & Layers & 0 & 1 & 2 & 4 \\
   \hline	
   ViT-B/16 & $224 \times 224$ & 12 & 89.7 & 90.8 & 92.1 & 93.0 \\
   ViT-B/16+ & $240 \times 240$ & 12 & 93.2 & 94.5 & 95.9 & 96.5 \\
   ViT-L/14 & $224 \times 224$ & 24 & 92.0 & 93.2 & 94.0 & 94.9 \\
    \bottomrule[1.5pt]
    \end{tabular} 
    }\vspace{-2mm}
\end{table}

\begin{figure*}[t]
    \centering 
    % \vspace{-4mm}
    \includegraphics[width=1\linewidth]{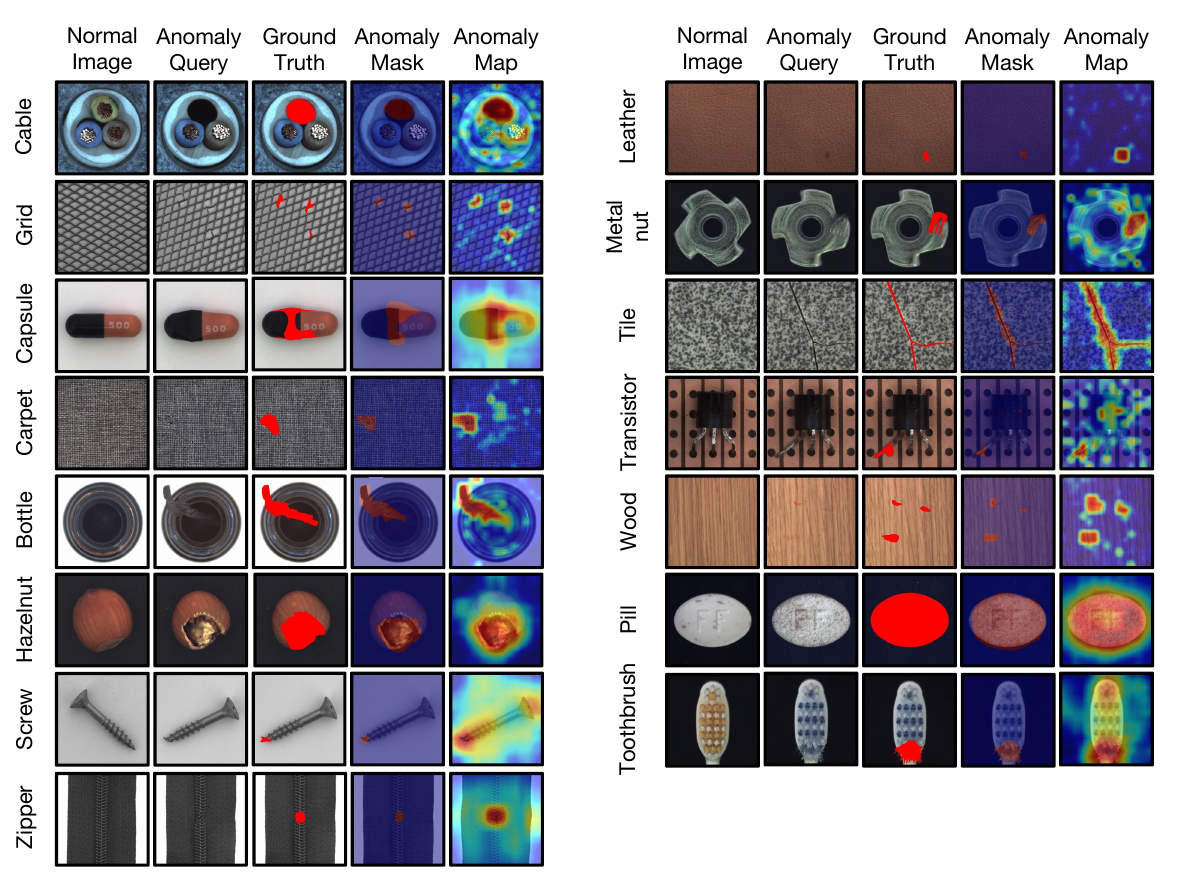}
    \caption{Detailed qualitative results of 0-shot visual anomaly detection on MVTec. The anomaly mask represents the binarized pixel-level anomaly map, where the annotated orange regions indicate detected anomalies.
    % Annotated orange regions indicate detected anomalies, showcasing effective localization of \name across diverse anomalies (e.g., broken, cracked, and bent of varying sizes and quantities) within various image classes.
    }
    \label{fig:visualization_mvtec_0}
    % \vspace{-2mm}
\end{figure*}

\section{Additional qualitative results}
\label{sec:add_visualizations}
In Figure~\ref{fig:visualization_mvtec_0}-\ref{fig:visualization_visa_4}, we present further qualitative results obtained from \name in the zero-shot and few-shot regime, showcasing diverse anomalies such as broken, cracked, structural changes, and bent instances of varying sizes and quantities. 
These results span various image classes from the MVTec and VisA benchmarks.
In Figure~\ref{fig:visualization_mvtec_0}-\ref{fig:visualization_visa_0}, we provide normal images for each class in benchmarks as reference points in order to facilitate a clearer identification of anomalies, which were not included as inputs in the model during the zero-shot experiments.

In the zero-shot regime, relying solely on language-driven \name demonstrates strong capabilities in generalizing to new and unseen anomalies, excelling in detecting common anomalies. 
However, in certain cases, assessing anomalies without a normal image reference proves challenging, such as anomalies that are very similar to normal samples. 
\name exhibits improved detection of finer, more domain-specific anomalies in the few-shot regime.
The combination of zero-shot capabilities for broad applicability and few-shot capabilities for domain-specific adaptation highlights the importance of striking a balance between generalization and specificity for effective anomaly detection.

\begin{figure*}[t]
    \centering 
    % \vspace{-4mm}
    \includegraphics[width=1\linewidth]{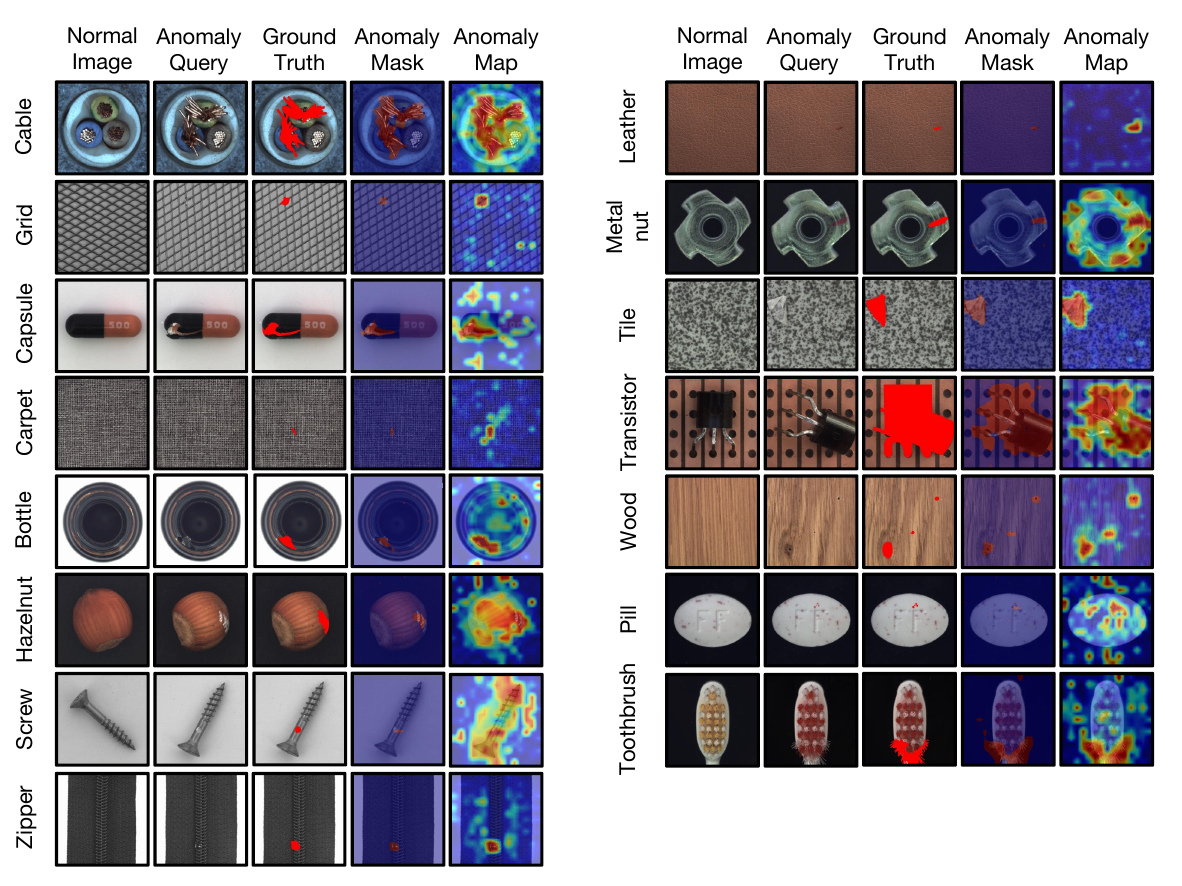}
    \caption{Detailed qualitative results of 4-shot visual anomaly detection on MVTec. The anomaly mask represents the binarized pixel-level anomaly map, where the annotated orange regions indicate detected anomalies.
    }
    \label{fig:visualization_mvtec_4}
    % \vspace{-2mm}
\end{figure*}

\begin{figure*}[t]
    \centering 
    % \vspace{-4mm}
    \includegraphics[width=1\linewidth]{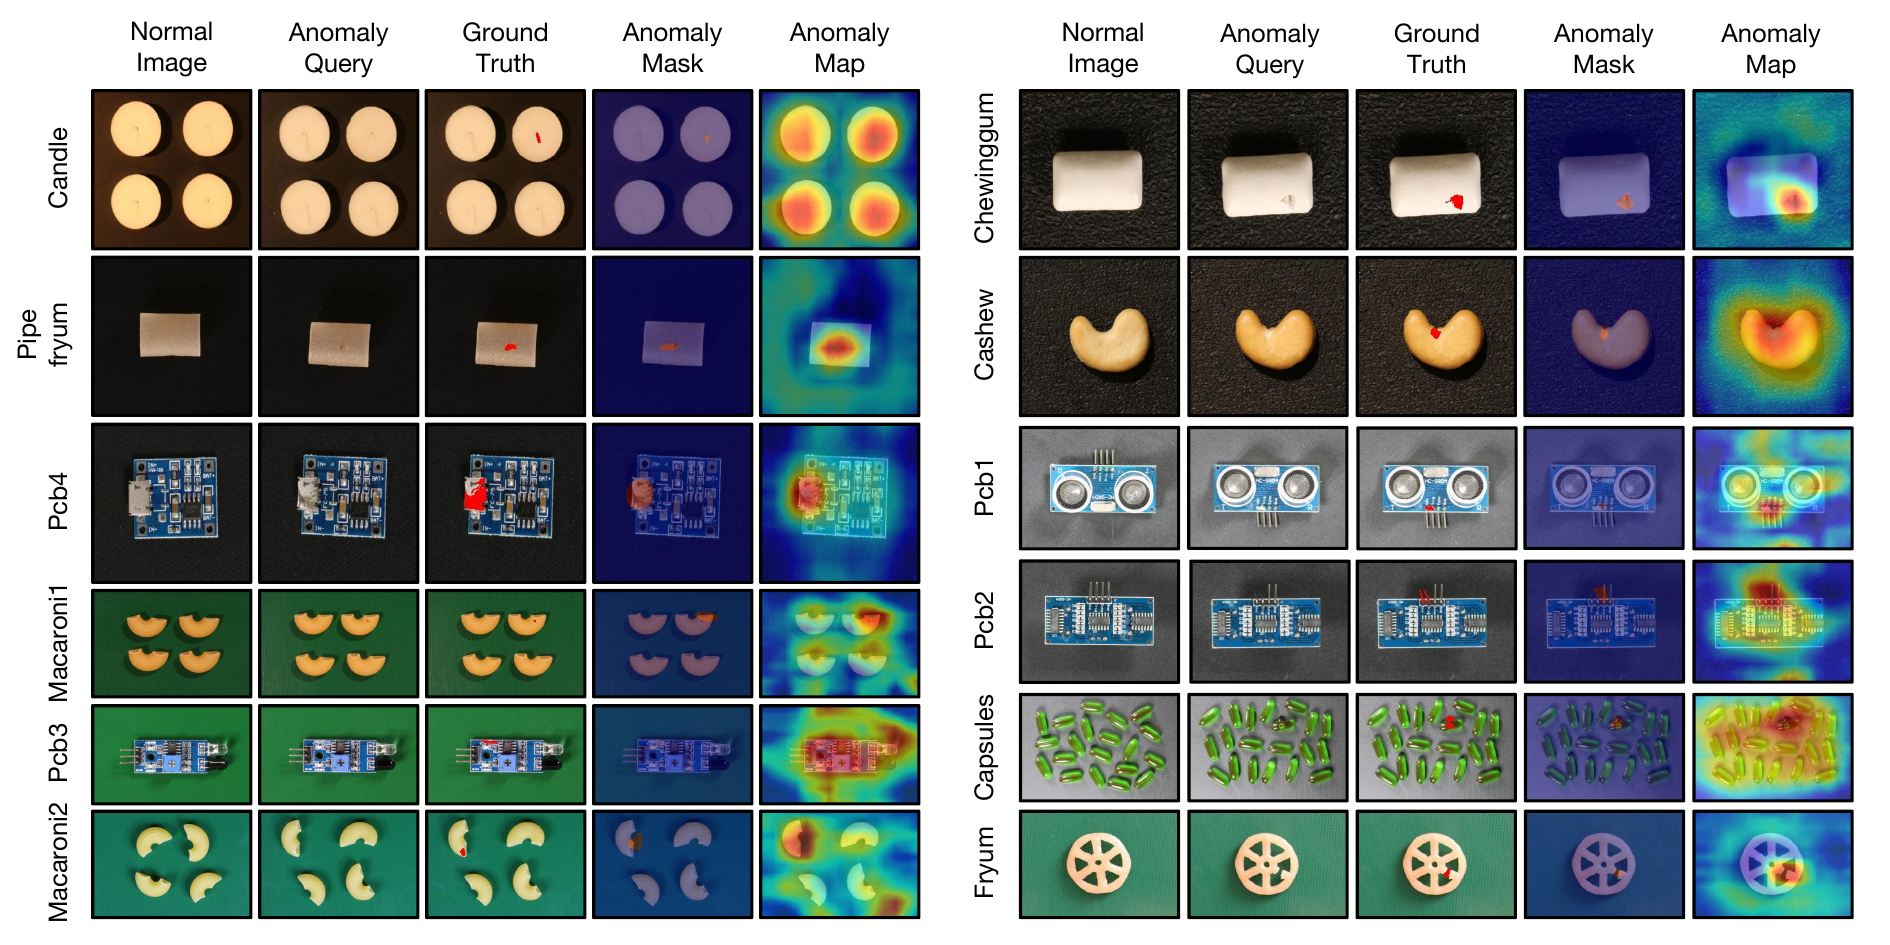}
    \caption{Detailed qualitative results of 0-shot visual anomaly detection on VisA. The anomaly mask represents the binarized pixel-level anomaly map, where the annotated orange regions indicate detected anomalies.
    }
    \label{fig:visualization_visa_0}
    % \vspace{-2mm}
\end{figure*}

\begin{figure*}[t]
    \centering 
    % \vspace{-4mm}
    \includegraphics[width=1\linewidth]{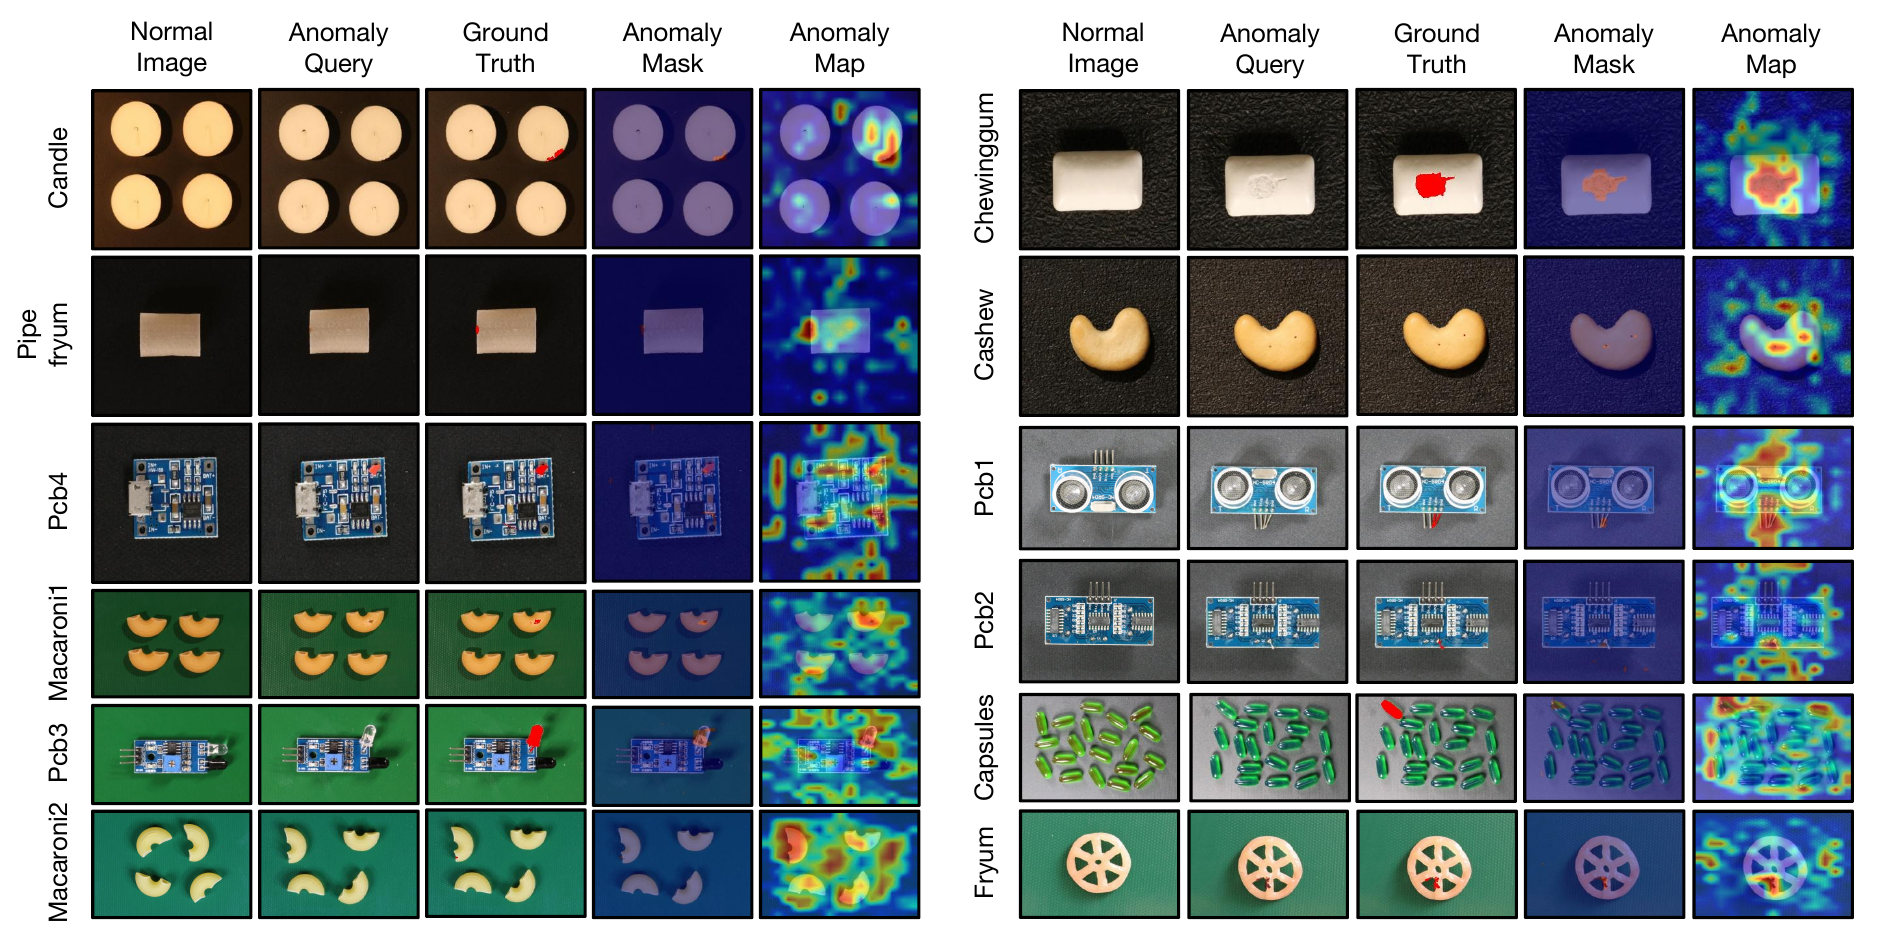}
    \caption{Detailed qualitative results of 4-shot visual anomaly detection on VisA. The anomaly mask represents the binarized pixel-level anomaly map, where the annotated orange regions indicate detected anomalies.
    }
    \label{fig:visualization_visa_4}
\end{figure*}
